# Supplementary material for: Stochastic Reconstruction of Gappy Lagrangian Turbulent Signals by Conditional Diffusion Models
Source: arXiv:2410.23971 source file (2024-10-31)
Supplement: Supplementary file 1 [file Supplementary_Information.pdf]

# Supplementary Information for "Stochastic Reconstruction of Gappy Lagrangian Turbulent Signals by Conditional Diffusion Models"

Tianyi Li[1], Luca Biferale[1], Fabio Bonaccorso[1], Michele Buzzicotti[1], and Luca Centurioni[2]
[1] *Department of Physics and INFN, University of Rome 'Tor Vergata', Via della Ricerca Scientifica 1, 00133 Rome, Italy and*
[2] *Lagrangian Drifter Laboratory, Scripps Institution of Oceanography, La Jolla, California, USA*
(Dated: October 24, 2024)

In this supplementary material, we apply Lagrangian turbulence reconstruction to a generic velocity component in two different scenarios to demonstrate the flexibility and robustness of our conditional diffusion model (C-DM). The first scenario involves interpolation, where measurements are sampled at fixed intervals. The second scenario explores the use of C-DM for prediction, where a gap is located at the right edge of the data. By iteratively using the predictions as inputs, we can extend the forecast over a very long time period, during which the model maintains stable statistical properties.

For the interpolation case, we consider sampling intervals of $10\tau_\eta$ and $20\tau_\eta$, corresponding to gaps between points of $9.9\tau_\eta$ and $19.9\tau_\eta$, respectively. Fig.1a shows the global mean squared error (MSE) from C-DM and Gaussian Process Regression (GPR) for these two sampling intervals. Although interpolation is relatively less challenging for GPR compared to gap filling, C-DM still manages to improve the MSE. In Fig.1b,c we show the marginal probability density functions (PDFs) of the stochastic reconstructions from C-DM and GPR for a fixed configuration (black) and a sampling interval of $20\tau_\eta$. The results are consistent with those in the main text, indicating that C-DM is able to capture the intermittency of the signal, while GPR only produces Gaussian predictions.

In Fig.2a, we show the MSE as a function of time within a right-end gap of size $100\tau_\eta$, demonstrating the consistent improvement of C-DM over GPR. As the gap lacks contextual information on the right, the MSE increases with time, eventually reaching approximately 2, signifying that the prediction is uncorrelated with the ground truth but still retains the correct second-order statistical properties (see Appendix D of [1] for a brief explanation). By iteratively shifting the prediction window to the right and using the predicted values as input for subsequent steps, we perform long-term predictions for all DNS test data. Fig.2d,e show the acceleration of the long-term forecasts from C-DM and GPR, respectively, both starting from a single initial measurement shown in black. The corresponding PDFs for these forecasts are shown on the right, where the C-DM result closely matches the DNS reference, while GPR gives a trivial Gaussian PDF. In Fig.2b, we present the generalized fourth-order flatness, $F_\tau^{(4)}$, for DNS and predictions made by C-DM and GPR over the interval $t \in [200\tau_\eta, 400\tau_\eta)$. It is evident that C-DM passes the quantitative multiscale test for this forecasting scenario. Fig.2c shows the flatness over different time intervals during the long-term forecasting using C-DM, demonstrating the robustness of the statistical properties as the self-iteration process continues.

[1] T. Li, M. Buzzicotti, L. Biferale, F. Bonaccorso, S. Chen, and M. Wan, Multi-scale reconstruction of turbulent rotating flows with proper orthogonal decomposition and generative adversarial networks, Journal of Fluid Mechanics **971**, A3 (2023).

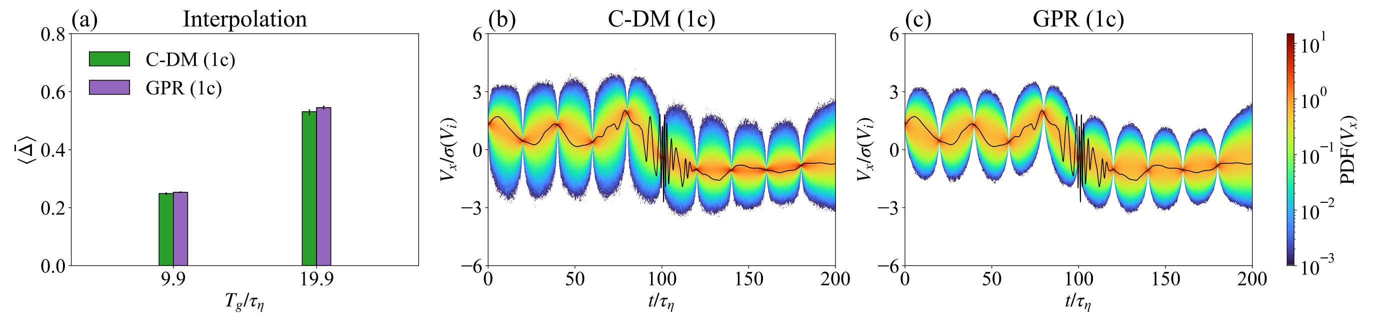


FIG. 1. (a) Bar plot of the overall MSE, $\langle\bar{\Delta}\rangle$, for Lagrangian turbulence interpolation, where the measurements are points sampled every $10\tau_0$ and $20\tau_0$, corresponding to gaps of size $9.9\tau_0$ and $19.9\tau_0$, respectively. Results are shown for a generic velocity component (1c) using C-DM (green bars) and Gaussian process regression (GPR, purple bars). (b,c) Marginal PDFs of the $x$ velocity component from stochastic reconstructions for Lagrangian turbulence interpolation with an equivalent gap size of $19.9\tau_0$ from GPR for the 1c case (b) and C-DM for the 1c case (c). The ground truth realization is shown as a black line for reference.

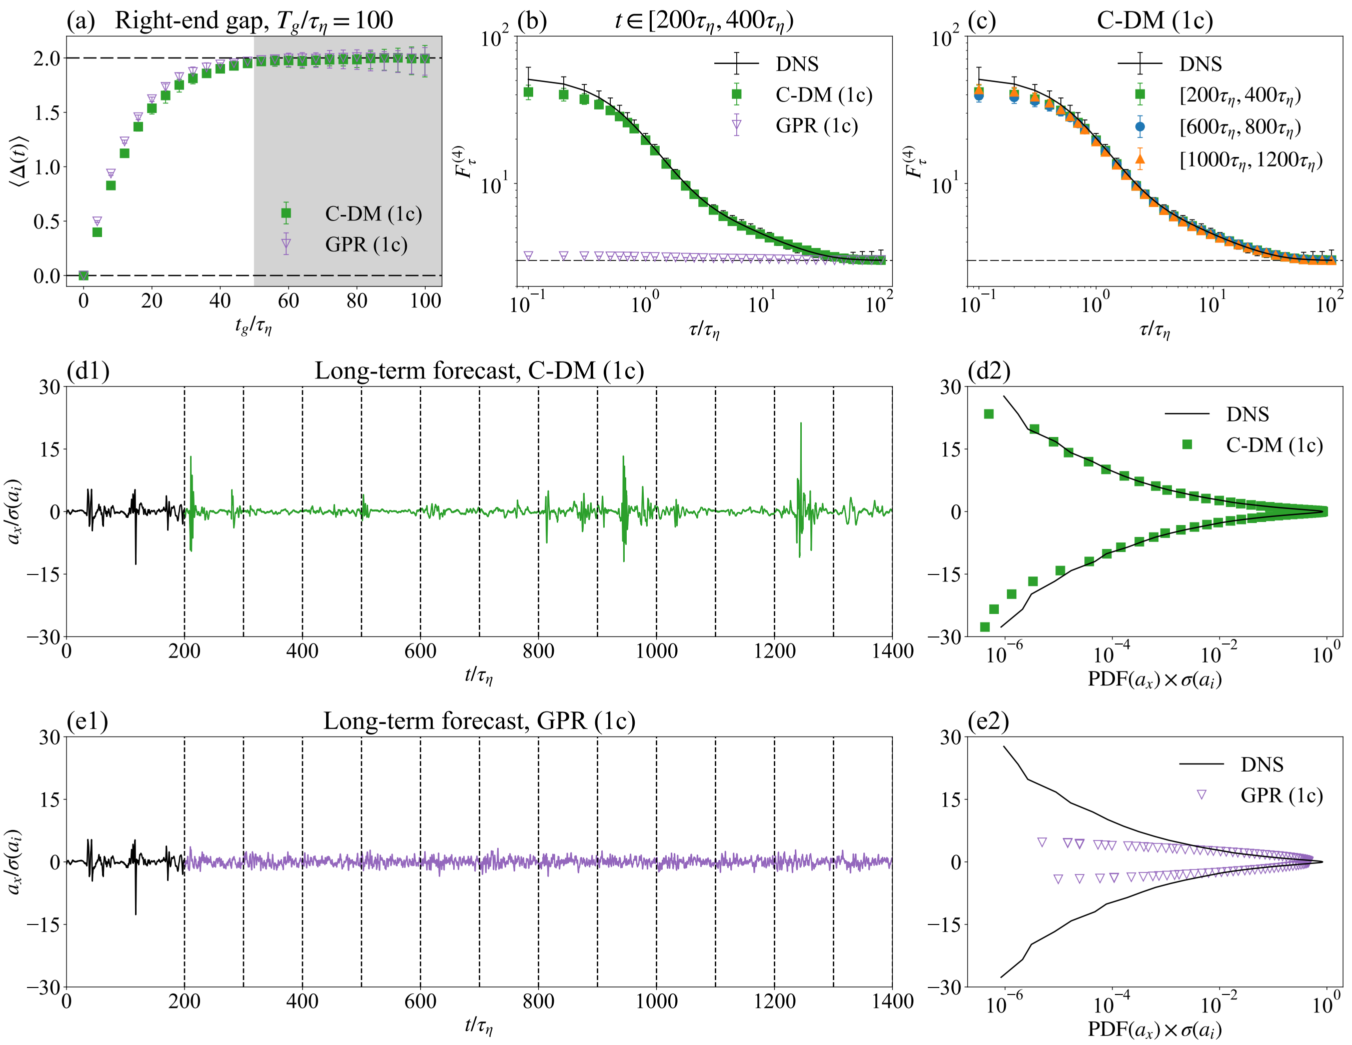


FIG. 2. (a) The MSE, $\langle\Delta(t)\rangle$, as a function of time within the gap for the Lagrangian turbulence reconstruction using C-DM and GPR for the 1c case, with a right-end gap size of $100\tau_\eta$. When $t_g \gtrsim 50\tau_\eta$, the MSE reaches a value around 2 (indicated by the gray region), indicating that the prediction is uncorrelated with the ground truth but still retains the correct second-order statistical properties. The gray region indicates where the MSE reaches the uncorrelated value of approximately 2. (b,c) Generalized fourth-order flatness, $F_\tau^{(4)}$, for DNS and predictions obtained by iteratively extending the reconstruction at the right end, starting from the DNS test configurations. Error bars are estimated from the spread across three batches, each belonging to the same velocity component of the test dataset. In panel b, forecasts are obtained from C-DM (1c) and GPR (1c) over the interval $t \in [200\tau_\eta, 400\tau_\eta)$. In panel c, forecasts are obtained from C-DM (1c) over different time intervals: $[200\tau_\eta, 400\tau_\eta)$, $[600\tau_\eta, 800\tau_\eta)$, and $[1000\tau_\eta, 1200\tau_\eta)$, demonstrating the roll-out stability of the statistical properties of C-DM. (d,e) Acceleration of long-term forecasts from C-DM (d1) and GPR (e1) for a generic velocity component, starting from the same initial configuration (black solid line), where the prediction window at each iteration is indicated by vertical black dashed lines. Panels (d2) and (e2) show the corresponding standardized PDFs, obtained from forecasting that specific configuration over the interval $t \in [200\tau_\eta, 205000\tau_\eta)$. The DNS result is shown for reference, derived from 1024 test data samples to ensure equivalent statistics.
